# Supplementary material for: Surfing: Iterative optimization over incrementally trained deep networks
Source: arXiv:1907.08653 source file (2019-07-19)
Supplement: Supplementary file 2 [file supplement.tex]

% !TEX root = surfing.tex

\section{Supplement: Proof of Theorem \ref{thm:init}}\label{sec:proof}
